# Supplementary material for: Disentangling Instance and Scene Contexts for 3D Semantic Scene Completion
Source: arXiv:2507.08555 source file (2025-07-11)
Supplement: Supplementary file 1 [file X_suppl.tex]

\clearpage
\setcounter{page}{1}
\maketitlesupplementary
\setcounter{section}{0}

\section{Appendix}

\subsection{Datasets and Metrics}

\noindent\textbf{Datasets.} Our experimental validation utilizes two benchmark datasets: SemanticKITTI~\cite{behley2019semantickitti} and SSC-Bench-KITTI-360~\cite{li2023sscbench}, which originate from the KITTI Odometry~\cite{odometry} and KITTI-360~\cite{KITTI360} platforms correspondingly. The experiments are conducted within a defined cuboid region extending $51.2$ meters ahead of the vehicle, $25.6$ meters laterally on both sides, and $6.4$ meters vertically. This spatial configuration is divided into discrete voxel grids of dimension $256\times256\times32$, with each cubic unit spanning $0.2$ meters per edge. For SemanticKITTI~\cite{behley2019semantickitti}, the framework processes RGB inputs sized at $1226\times370$ pixels, annotated with $20$ distinguishable semantic labels ($19$ object categories and $1$ void class). The dataset partitioning comprises $10$ training sequences, $1$ validation sequence, and $11$ testing sequences. The SSC-Bench-KITTI-360 variant~\cite{li2023sscbench} delivers higher-resolution $1408\times376$ RGB imagery containing $19$ class labels ($18$ semantic types and $1$ free space), with its data split structured as $7$ training sequences, $1$ validation sequence, and $1$ testing sequence.

\noindent\textbf{Category Partitioning.} We categorize the classes in SemanticKITTI and SSC-Bench-KITTI-360 datasets into instance and scene groups based on commonsense criteria. For SemanticKITTI, instance categories include: \emph{car, bicycle, motorcycle, truck, other-vehicle, person, bicyclist, motorcyclist, pole, and traffic-sign}. Scene categories comprise: \emph{road, parking, sidewalk, other-ground, building, fence, vegetation, trunk, and terrain}. In SSC-Bench-KITTI-360, instance classes are defined as \emph{car, bicycle, motorcycle, truck, other-vehicle, person, pole, traffic-sign, and other-object}, while scene classes consist of \emph{road, parking, sidewalk, other-ground, building, fence, vegetation, terrain, and other-structure.}

\noindent\textbf{Metrics.} Following established practices in~\cite{yu2024context,jiang2024symphonize,cao2022monoscene,li2023voxformer,huang2023tri}, we adopt intersection over union (IoU) for occupied voxel grids and mean IoU (mIoU) for voxel-wise semantic predictions as evaluation metrics. To enable differentiated analysis of instance and scene categories, we further introduce Instance mIoU (InsM) and Scene mIoU (ScnM). These specialized metrics are computed by averaging IoU scores exclusively over their respective category groups (instance-related or scene-related classes). This dual-metric framework provides granular insights into the model's predictive capabilities across distinct semantic categories.

\subsection{Implementation Details}
\noindent\textbf{Network Structures.} Following Symphonies, we employ a ResNet-50~\cite{resnet} image backbone and an Instance-Aware Deformable Transformer~\cite{zhu2020deformable} encoder to extract 2D image features. A coarse-to-fine BEV module generates BEV feature maps with dimensions of $128\times128$ and $128$ channels. These BEV features are then split into instance BEV features and scene BEV features through multi-layer $3\times3$ convolutions, both retaining the same dimensions and channel count as the original BEV features.The instance and scene BEV features are fed into the DACD module, which contains three AIL layers and three GSL layers. The output BEV features are upsampled using predicted height information to generate instance volume and scene volume, each with dimensions $128\times128\times16$. These volumes are fused and passed into the 3D Local and Global Encoder adopted from CGFormer~\cite{yu2024context}, with the original BEV feature space encoder operations in the Global Encoder removed in our implementation. The final fused volume retains dimensions of $128\times128\times16$. Subsequently, upsampling is applied to increase the resolution to $256\times256\times32$ for alignment with ground truth. A prediction head is finally used to produce the output.

\noindent\textbf{Training Setup.} We train DISC using $4$ NVIDIA $3090$ GPUs with a batch size of $4$. The training process consumes approximately $16$ GB of GPU memory per GPU. We set the total training epochs to $20$ and adopt an EarlyStopping strategy to reduce training time. The AdamW optimizer is employed with an initial learning rate of $1.0\times10^{-2}$, which is reduced by a factor of $10$ at the $12$th epoch.

\begin{table*}[ht]
    \centering
    \newcommand{\clsname}[2]{
        \rotatebox{90}{
            \hspace{-6pt}
            \textcolor{#2}{$\blacksquare$}
            \hspace{-6pt}
            \renewcommand\arraystretch{0.6}
            \begin{tabular}{l}
                #1                                      \\
                \hspace{-4pt} ~\tiny(\semkitfreq{#2}\%) \\
            \end{tabular}
        }}

    \renewcommand\arraystretch{1.1}
    \resizebox{\linewidth}{!}
    {
        \begin{tabular}{l|r>{\columncolor{gray!20}}rrr|rrrrrrrrrrrrrrrrrrrr}
            \toprule
            Method                               &
            \multicolumn{1}{c}{IoU}              &
            mIoU             &
            \multicolumn{1}{c}{InsM}             &
            ScnM                                 &

            \clsname{road}{road}                 &
            \clsname{sidewalk}{sidewalk}         &
            \clsname{parking}{parking}           &
            \clsname{other-grnd.}{otherground}   &
            \clsname{building}{building}         &
            \clsname{car}{car}                   &
            \clsname{truck}{truck}               &
            \clsname{bicycle}{bicycle}           &
            \clsname{motorcycle}{motorcycle}     &
            \clsname{other-veh.}{othervehicle}   &
            \clsname{vegetation}{vegetation}     &
            \clsname{trunk}{trunk}               &
            \clsname{terrain}{terrain}           &
            \clsname{person}{person}             &
            \clsname{bicyclist}{bicyclist}       &
            \clsname{motorcyclist}{motorcyclist} &
            \clsname{fence}{fence}               &
            \clsname{pole}{pole}                 &
            \clsname{traf.-sign}{trafficsign}
            \\
            \midrule
			MonoScene$^\ast$~\cite{cao2022monoscene} & 36.86 & 11.08 & 4.22 & 18.69 & 56.52 & 26.72 & 14.27 & 0.46  & 14.09 & 23.26 & 6.98  & 0.61  & 0.45  & 1.48  & 17.89 & 2.81  & 29.64 & 1.86  & 1.20  & 0.00  & 5.84  & 4.14  & 2.25 \\
			TPVFormer~\cite{huang2023tri}  & 35.61 & 11.36 & 4.27 & 19.24 & 56.50 & 25.87 & 20.60 & 0.85  & 13.88 & 23.81 & 8.08  & 0.36  & 0.05  & 4.35  & 16.92 & 2.26  & 30.38 & 0.51  & 0.89  & 0.00  & 5.94  & 3.14  & 1.52 \\
			OccFormer~\cite{zhang2023occformer} & 36.50 & 13.46 & 7.39 & 20.20 & 58.85 & 26.88 & 19.61 & 0.31  & 14.40 & 25.09  & \textbf{25.53} & 0.81  & 1.19  & 8.52  & 19.63 & 3.93  & 32.62 & 2.78  & 2.82  & 0.00  & 5.61  & 4.26  & 2.86 \\
			IAMSSC~\cite{xiao2024instance}  & 44.29 & 12.45 & 5.55 & 20.12 & 54.55 & 25.85 & 16.02 & 0.70  & 17.38 & 26.26 & 8.74  & 0.60  & 0.15  & 5.06  & 24.63 & 4.95  & 30.13 & 1.32  & 3.46  & \underline{0.01}  & 6.86  & 6.35  & 3.56 \\
			VoxFormer-S~\cite{li2023voxformer}  & 44.02 & 12.35 & 5.27 & 20.23 & 54.76 & 26.35 & 15.50 & 0.70  & 17.65 & 25.79 & 5.63  & 0.59  & 0.51  & 3.77  & 24.39 & 5.08  & 29.96 & 1.78  & 3.32  & 0.00  & 7.64  & 7.11  & 4.18 \\
			VoxFormer-T~\cite{li2023voxformer}  & 44.15 & 13.35  & 6.14 & 21.37 & 53.57 & 26.52 & 19.69 & 0.42 & 19.54 & 26.54 & 7.26 & 1.28 & 0.56 & 7.81 & 26.10 & 6.10 & 33.06 & 1.93 & 1.97 & 0.00 & 7.31 & 9.15 & 4.94 \\
			DepthSSC~\cite{yao2023depthssc}  & 45.84 & 13.28 & 6.14 & 20.21 & 55.38 & 27.04 & 18.76 & 0.92  & 19.23 & 25.94 & 6.02  & 0.35  & 1.16  & 7.50  & 26.37 & 4.52  & 30.19 & 2.58  & \textbf{6.32}  & 0.00  & 8.46  & 7.42  & 4.09 \\
			Symphonize~\cite{jiang2024symphonize}  & 41.92 & 14.89 & \underline{8.94} & 21.49 & 56.37 & 27.58 & 15.28 & 0.95  & 21.64 & 28.68 & \underline{20.44} & 2.54  & 2.82  & \textbf{13.89} & 25.72 & 6.60  & 30.87 & 3.52  & 2.24  & 0.00  & 8.40  & 9.57  & 5.76 \\
			HASSC-S~\cite{wang2024not}  & 44.82 & 13.48 & 3.68 & 21.38 & 57.05 & 28.25 & 15.90 & 1.04 & 19.05 & 27.23 & 9.91 & 0.92 & 0.86 & 5.61 & 25.48 & 6.15 & 32.94 & 2.80 & 4.71 & 0.00 & 6.58 & 7.68 & 4.05 \\
			HASSC-T~\cite{wang2024not} & 44.58 & 14.74 & 5.27 & 24.51 & 55.30 & 29.60 & \underline{25.90} & \textbf{11.30} & 23.10& 23.00 & 2.90 & 1.90 & 1.50 & 4.90 & 24.80 & 9.80 & 26.50 & 1.40 & 3.00 & 0.00 & \textbf{14.30} & 7.00 & 7.10 \\ 
			H2GFormer-S~\cite{wang2024h2gformer} & 44.57 & 13.73 & 6.36 &  21.99 & 56.08 & 29.12 & 17.83 & 0.45 & 19.74 & 28.21 & 10.00 & 0.50 & 0.47 & 7.39 & 26.25 & 6.80 & 34.42 & 1.54 & 2.88 & 0.00 & 7.24 & 7.88 & 4.68 \\
			H2GFormer-T~\cite{wang2024h2gformer}  & 44.69 & 14.29 & 6.31 & 23.16 & 57.00 & 29.37 & 21.74 & 0.34 & 20.51 & 28.21 & 6.80 & 0.95 & 0.91 & 9.32 & \underline{27.44} & 7.80 & 36.26 & 1.15 & 0.10 & 0.00 & 7.98 & 9.88 & 5.81 \\
            VPOcc~\cite{kim2024vpocc} &44.5 &15.59	&8.93	&22.99 & 58.46 & 28.61 & 17.91 & 0.36 & \textbf{24.88} & 30.42 & 18.51 & 2.82 & \textbf{3.88} & \underline{13.85} & 27.14 & 6.36 & 33.98 & 3.7 & 2.36 & \textbf{0.23} & 9.19 & 8.55 & 4.98 \\
			CGFormer~\cite{yu2024context}   & \textbf{45.99} & \underline{16.87} & \textbf{9.372} & \underline{25.20} & \textbf{65.51} & \underline{32.31} & 20.82 & 0.16  & 23.52 & \textbf{34.32}
			& 19.44 & \textbf{4.61} & 2.71  & 7.67  & 26.93 & \textbf{8.83} & \underline{39.54} & 2.38  & 4.08  & 0.00  & 9.20 & \underline{10.67} & \textbf{7.84} \\
            \hline
            \textbf{DISC(Ours)} & \underline{45.93} & \textbf{17.05} & 8.755 & \textbf{26.27} & \underline{64.32} & \textbf{34.6}	& \textbf{26.93}	& \underline{1.45}	& \underline{23.77}	& \underline{33.07} & 11.78 & \underline{3.02} & 3.27	& 9.50 	& \textbf{27.77}	 & 7.88	& \textbf{39.79}	& \textbf{4.2} & \underline{4.72} & 0.00 & \underline{9.91} & \textbf{10.86} & \underline{7.13}\\
            \bottomrule
        \end{tabular}
    }
    \caption{\textbf{Quantitative results on SemanticKITTI \texttt{val}.} $^\ast$ represents the reproduced results from~\cite{huang2023tri,zhang2023occformer}.The best-performing method among all approaches is highlighted in \textbf{bold}, while the second-best is marked with an \underline{underline}.}
    \label{tab:sem_kitti_val}
\end{table*}

% \subsection{Details of Position Embedding.}
% The BEV plane serves as the primary feature interaction space, where all queries, including image queries, have their positional embeddings determined by the projection points $P(x, y)$ on the BEV plane. By using a predefined BEV plane range, $x$ and $y$ are normalized to obtain $x_n$ and $y_n$, which are then encoded into high-dimensional embeddings using sine and cosine functions. Subsequently, two linear layers, followed by ReLU and LayerNorm, are applied to process the learnable pose embeddings.

\subsection{Details of Coarse-to-fine BEV Generation} BEV features, enriched with semantic and geometric priors, play a crucial role in aggregating both instance and background information. Previous works~\cite{philion2020lift,li2022bevformer} have proposed various methods for obtaining BEV features, with the Lift-Splat paradigm standing out for its simplicity and computational efficiency. However, this approach is highly sensitive to the accuracy of depth predictions~\cite{li2022bevformer} and fails to fully utilize the available depth information. 

To address these limitations, the Coarse-to-Fine BEV Generation module extends the Lift-Splat approach, fully leveraging known depth information to mitigate geometric ambiguities that impact downstream tasks. In our method, the Lift operation first extracts depth distributions $\mathbf{D} \in \mathbb{R}^{H \times W \times D}$ and contextual features $\mathbf{C} \in \mathbb{R}^{H \times W \times C}$ from $F^{2D}$, where $(H, W)$ denotes the image resolution and $D$ represents the number of discrete depths. These are then used to derive the camera frustum features, which are subsequently transformed into coarse voxel features $V_{\text{coarse}}$ through a camera-to-world transformation, as described below:
\begin{equation}
    V_{\text{coarse}} = \mathcal{T}^{CW}(\mathbf{D}\odot \mathbf{C})
\end{equation}
Here, $\mathcal{T}^{CW}$ refers to the camera-to-world transformation and $\odot$ represents the scaling and propagation operations of the contextual features along the depth direction, as described in~\cite{philion2020lift}.

Since each pixel in the image plane corresponds to a known depth value, the voxels located on the implicit surface, known as voxel proposals, have their coordinates $X_p$ obtained through $\mathcal{T}^{CW}$:
\begin{align}
    {X}_p &= \left\{ x^W \;\middle|\; x^W = \mathcal{T}^{CW}(x^C), \right. \nonumber \\
    &\qquad \qquad\left. \forall x^C \in X_c \text{ such that } x^W \in X_v \right\}
\end{align}
where $x^C$ and $x^W$ represent the coordinates of the proposed voxel points in the camera and world coordinate systems, respectively, while $X_c$ and $X_v$ denote the corresponding coordinate sets in the camera space and predefined voxel space. Based on this, the initial feature $\mathbf{Q}_p^{c} \in \mathbb{R}^{P \times C}$ of the proposed voxels, where $P$ denotes the number of proposed voxels, is derived through coordinate selection from $V_{\text{coarse}}$. Mathematically, this can be expressed as follows:
\begin{align}
    \mathbf{Q}_p^{c} &= V_{\text{coarse}}[{X}_p] 
\end{align}
Inspired by~\cite{jiang2024symphonize}, $\mathbf{Q}_p^{c}$ interacts with the multi-scale image features $F^{2D}$ through Deformable Attention~\cite{zhu2020deformable} to obtain $\mathbf{Q}_p^{f} \in \mathbb{R}^{P \times C}$, which captures more fine-grained semantic information. The formula is expressed as:
\begin{equation}
    \mathbf{Q}_p^{f} = \text{DA}(\mathbf{Q}_p^{c}, F^{2D}, p_I) = \sum_{k=1}^K A_k W \phi(F^{2D}, p_I + \Delta p)
\end{equation}
Here, $K$ represents the number of sampled points, $A_k$ denotes the learnable sampling weights, and $W$ refers to the projection weights. $p_I$ refers to reference points in the image space, while $\Delta p$ represents the offset relative to $p_I$. $\phi(F^{2D}, p_I + \Delta p)$ indicates feature sampling in image space. Furthermore, $V_{\text{fine}}$ is obtained by replacing $\mathbf{Q}_p^{c}$ in $V_{\text{coarse}}$ with $\mathbf{Q}_p^{f}$.The BEV features $C_{\text{bev}}$ are obtained by pooling $V_{\text{fine}}$, followed by convolution applied on $C_{bev}$ to generate the initial $C_{\text{ins}}$ and $C_{\text{bk}}$, as described below:
\begin{equation}
    C_{\text{ins}} = \text{Conv}_{\text{ins}}(\text{Pooling}_{ \{z\}}(V_{\text{fine}}))
\end{equation}
\begin{equation}
    C_{\text{bk}} = \text{Conv}_{\text{bk}}(\text{Pooling}_{ \{z\}}(V_{\text{fine}}))
\end{equation}
where $\text{Pooling}_{ \{z\}}$ refers to the pooling operation along the Z-axis, consistent with that used in~\cite{yu2024context}.

Compared to the fixed voxel embeddings used for voxel feature initialization in~\cite{jiang2024symphonize}, the Lift method generates voxel features with coarse contextual information, enabling $\mathbf{Q}_p^{c}$ in Deformable Attention to more effectively integrate relevant semantic features. Furthermore, voxels within $X_v$ but not included in $X_p$ still retain the semantic information captured during the Lift process.

\begin{figure*}[htbp] %H为当前位置，!htb为忽略美学标准，htbp为浮动图形
    \centering
    \includegraphics[width=1\textwidth]{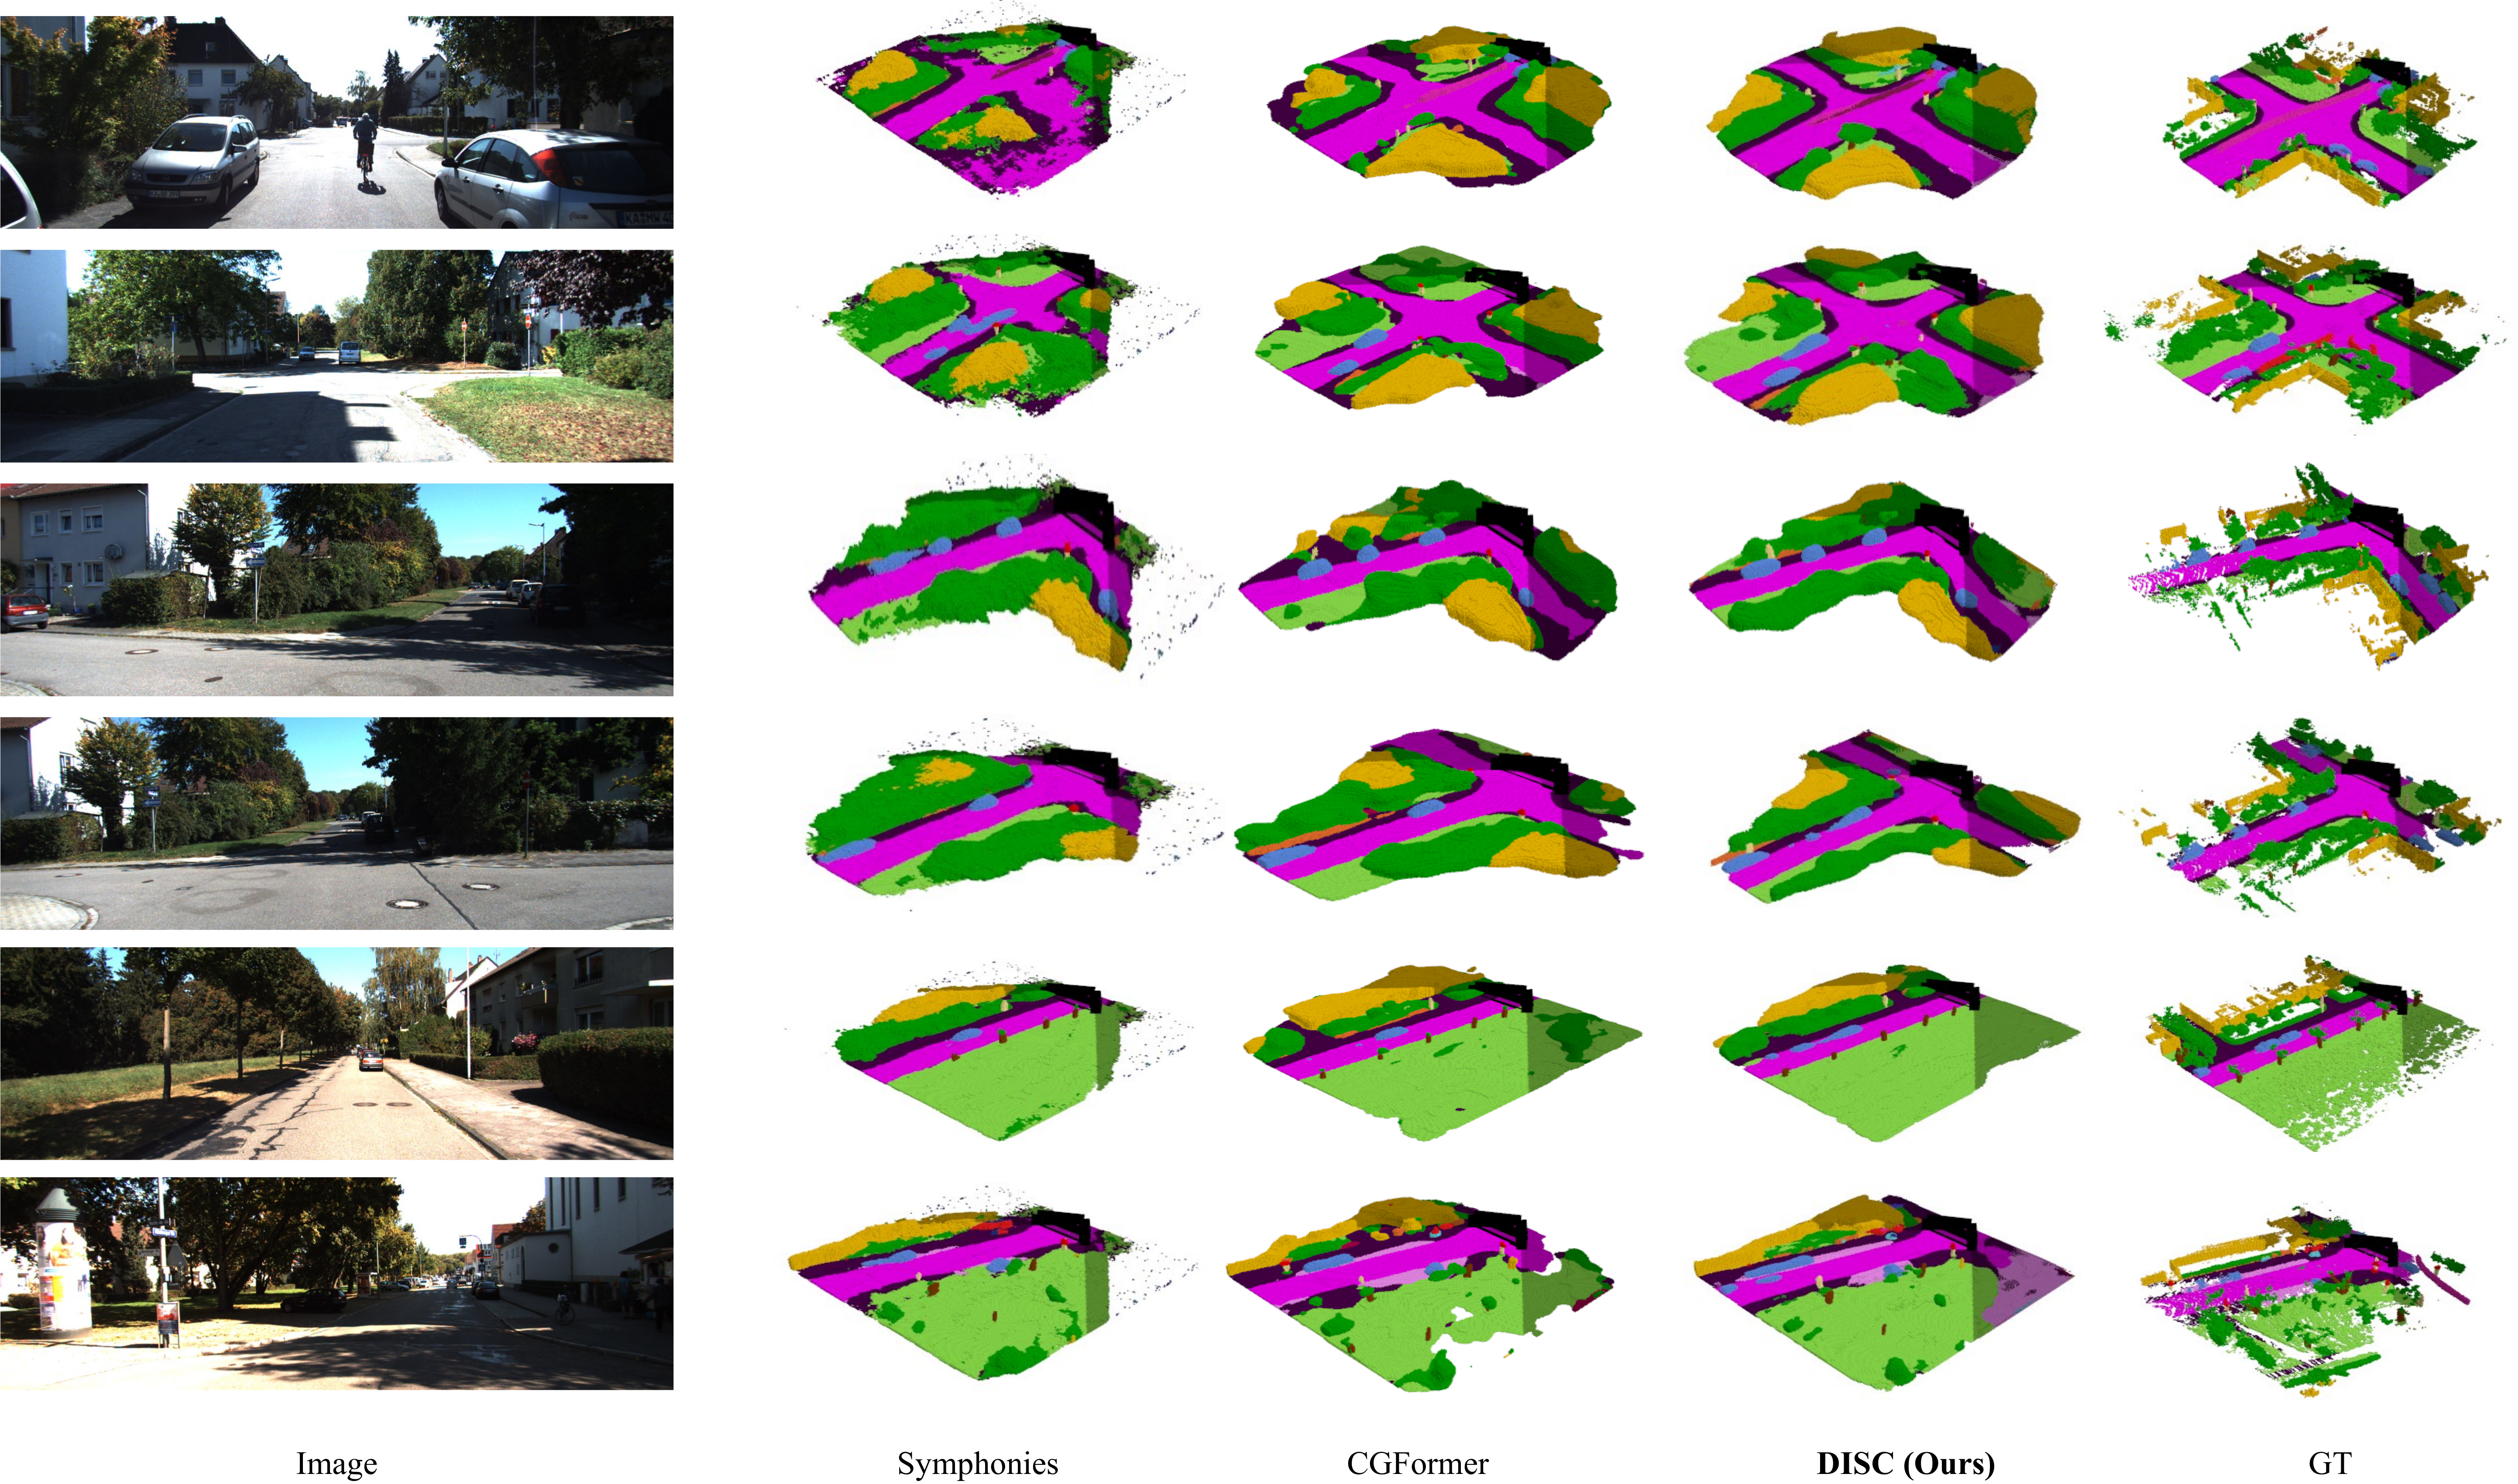}
    % \vspace{-10mm}
    \caption{\textbf{More qualitative visualization results on the SemanticKITTI~\cite{behley2019semantickitti} validation set.}}
    \label{su_vis_v2}
\end{figure*}

\subsection{Details of Position Embedding.}
The BEV plane serves as the primary feature interaction space, where all queries, including image queries, have their positional embeddings determined by the projection points $P(x, y)$ on the BEV plane. By using a predefined BEV plane range, $x$ and $y$ are normalized to obtain $x_n$ and $y_n$, which are then encoded into high-dimensional embeddings using sine and cosine functions. Subsequently, two linear layers, followed by ReLU and LayerNorm, are applied to process the learnable pose embeddings.

\subsection{Ablation on Scene Query.} We conduct experiments on scene query patch size, with results illustrated in \cref{5-bkq}. Specifically, we test patch sizes of $2$, $4$, $16$, and $32$, and report the corresponding mIoU and ScnM scores under each configuration. Our analysis reveals that both ScnM and mIoU achieve optimal performance when the patch size is set to $4$. This observation can be attributed to the trade-off between local and global information: excessively small patch sizes lose global contextual information, while overly large ones introduce excessive local noise, thereby blurring class boundaries.

\begin{table}[ht]
    \centering
     % 设置灰色语法
    {
        \begin{tabular}{c|c>{\columncolor{gray!20}}c}
            \toprule

            Method   & \multicolumn{1}{c}{InsM$\uparrow$} & \multicolumn{1}{>{\columncolor{gray!20}}c}{mIoU$\uparrow$} \\
            \midrule
            vanilla Ins.-Img. CA         &  8.67   &  16.85      \\
            height-adaptive Ins.-Img. CA(Ours) & \textbf{8.75}  & \textbf{17.05}   \\
            \bottomrule
        \end{tabular}
    }
    \vspace{-0.1cm}
    \caption{\textbf{Ablation study on Instance-Image cross attention.} High-level features facilitate instance-image cross attention.}
    % \vspace{-0.1cm}
    \label{tab:abla_adH}
\end{table}
\subsection{Ablation on Instance-Image Cross Attention.} As shown in \cref{tab:abla_adH}, we compare the performance of the traditional instance-image cross-attention mechanism~\cite{li2022bevformer} with our proposed height-adaptive instance-image cross-attention. The latter achieves higher InsM and mIoU by 0.08 and 0.2, respectively, confirming that adaptive interaction along the height direction enhances instance reasoning.

\begin{figure}[!t]
    \centering
    \includegraphics[width=1.0\linewidth]{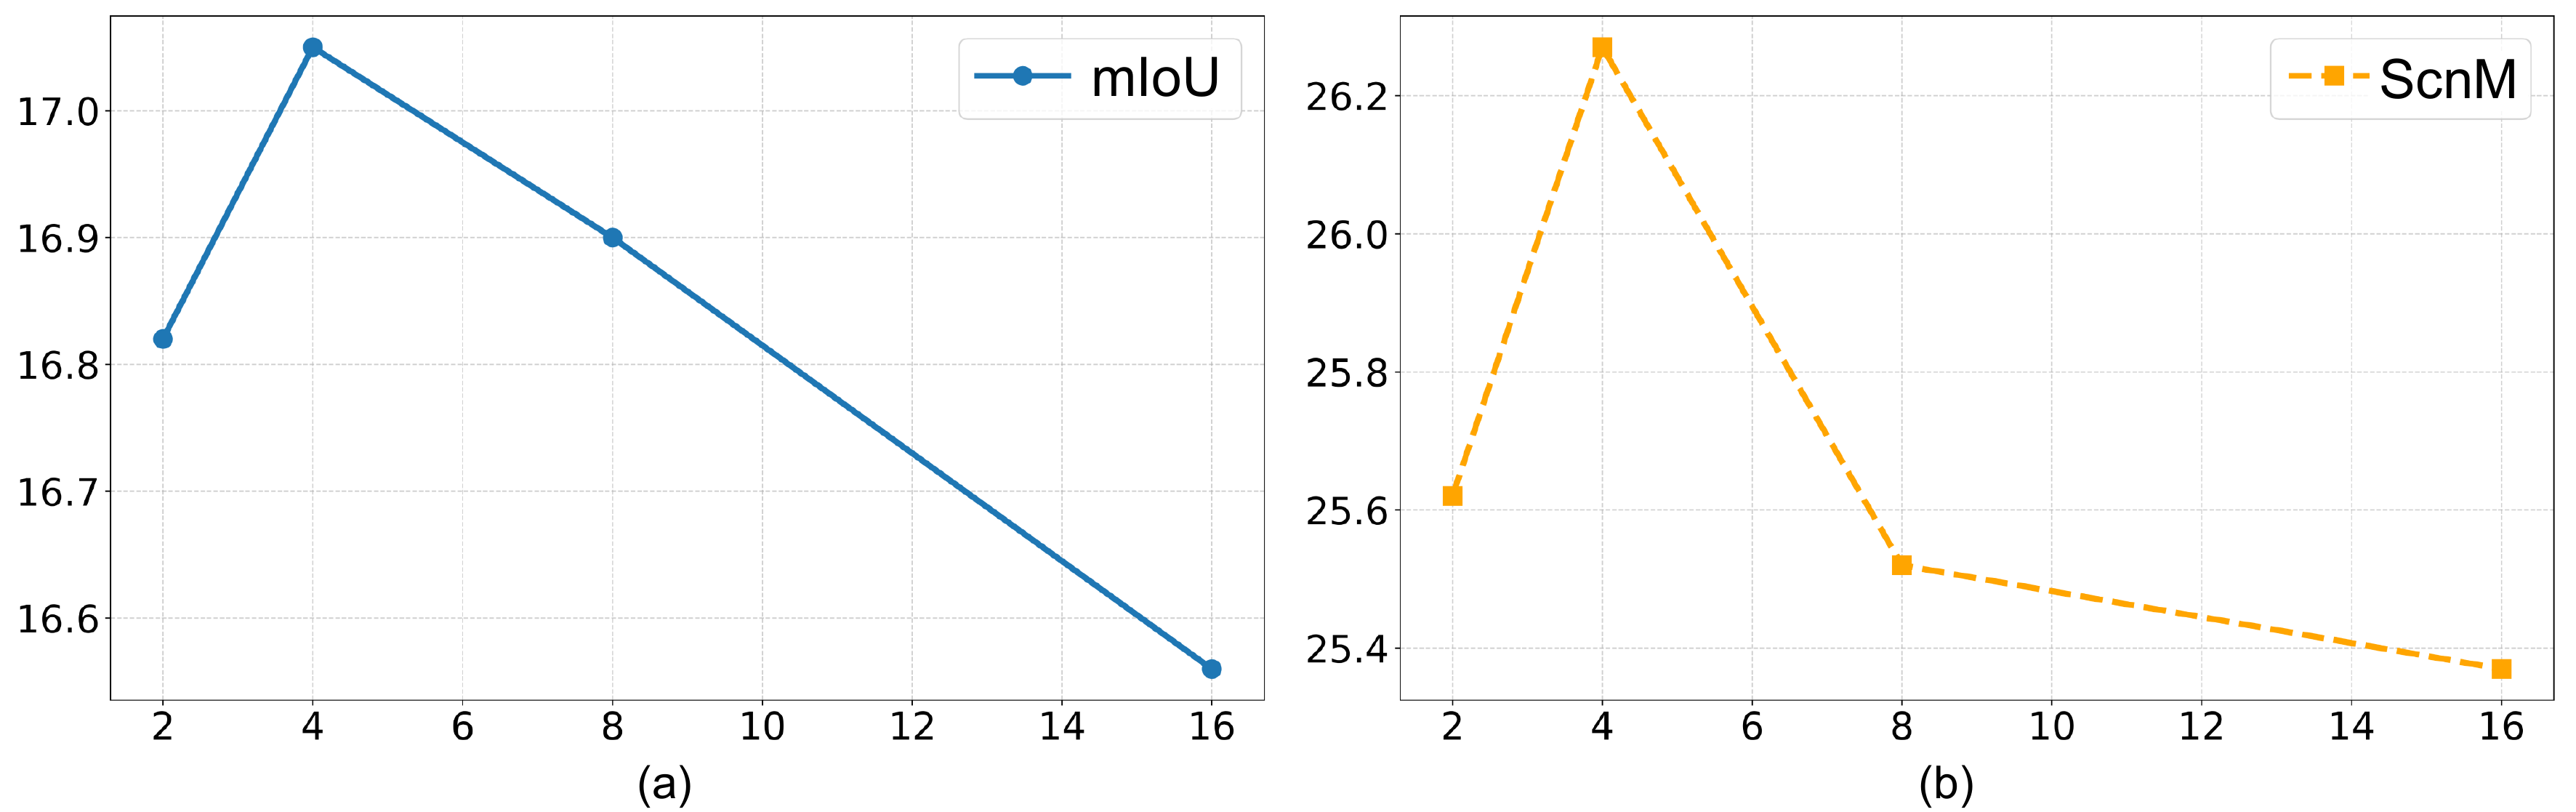}
    \vspace{-0.7cm}
    \caption{\textbf{Ablation study on scene query. }We investigate the impact of patch size during the initialization of scene queries on the quantitative metrics mIoU (a) and ScnM (b).}
    \vspace{-0.3cm}
    \label{5-bkq}
\end{figure}

\subsection{Results on SemanticKITTI val} In \cref{tab:sem_kitti_val}, we further provide quantitative results of DISC on the SemanticKITTI val set for a more comprehensive comparison. DISC remains the state-of-the-art (SOTA) method, demonstrating significant advantages in both instance and scene categories.

\subsection{More Visualizations} More visualization results are provided in \cref{su_vis_v2}, where we primarily compare with two state-of-the-art methods: Symphonies~\cite{jiang2024symphonize} and CGFormer~\cite{yu2024context}. These examples are randomly selected from the SemanticKITTI~\cite{behley2019semantickitti} validation set. The visual comparisons further validate that our method demonstrates stronger capability in capturing category-specific information for both instance and scene.
